# Supplementary material for: Asymptotically well-balanced geostrophic reconstruction finite volumes numerical schemes for the 2D rotating NLSWE in spherical coordinates
Source: arXiv:2510.16002 ancillary file (2025-10-14)
Supplement: Supplementary file 1 [file supplementary.pdf]

# SUPPLEMENTARY MATERIALS: ASYMPTOTICALLY WELL-BALANCED GEOSTROPHIC RECONSTRUCTION FINITE VOLUMES NUMERICAL SCHEMES FOR THE 2D ROTATING NLSWE IN SPHERICAL COORDINATES*

A. GONZÁLEZ †, M.J. CASTRO †, AND J. MACÍAS †

**SM1. Definition of the fluctuation function for the 1D system of balanced laws used in the numerical schemes.** The 2D fluctuation function defined in (3.2) relies upon the definition of a 1D fluctuation function $\mathcal{D}^-$ associated to the following 1D hyperbolic system:

$$\partial_t U_\sigma + \partial_x F(U_\sigma) + T^p(h)\partial_x \eta_\sigma = 0, \tag{SM1.1}$$

where $F(U_\sigma)$ and $T^p(h)$ are those in (2.7), and the rotational invariance-like properties (2.4) have been used. System (SM1.1) is a 1D shallow water system with gravity constant $\frac{g}{\sigma}$ and a transport equation for the tangential velocity $\frac{Q_{\vec{\nu}^\perp}}{h_\sigma}$. Adopting the strategy proposed in [SM3, SM2], we consider a polynomial viscosity method (PVM)

(SM1.2)

$$\begin{aligned}\mathcal{D}^-(U_{\sigma,L},\eta_{\sigma,L};U_{\sigma,R},\eta_{\sigma,R}) =& \frac{1}{2}\Big(F(U_{\sigma,R}) - F(U_{\sigma,L}) + T^p(h_{1/2})(\eta_{\sigma,R}-\eta_{\sigma,L})\Big)\\ &-\frac{1}{2}Q_{1/2}\Big(U_{\sigma,R}-U_{\sigma,L}\\ &+J_F^{-1}(U_{\sigma,L},U_{\sigma,R})T^p(h_{1/2})(\eta_{\sigma,R}-\eta_{\sigma,L})\Big)\end{aligned}$$

where $h_{1/2} = \frac{h_L+h_R}{2}$, $J_F(U_{\sigma,L},U_{\sigma,R})$ is the standard Roe matrix for system (SM1.1), and $Q_{1/2}$ is a viscosity matrix computed as $Q_{1/2} = P_n(J_F)$, for a given polynomial $P_n(x) = \sum_{j=0}^{n} a_j^{1/2} x^j$. This method is path-conservative for the family of paths given by the strait segments [SM6]. The PVM technique [SM1, SM5] defines numerical viscosity based on general polynomial evaluations of a Roe matrix. The definition of the polynomial $P_n$ leads to different numerical schemes, some of them well-known such as Roe method, HLL [SM4] or HLLC [SM7], among others. In particular, the 1D solver used here coincides with the one described in [SM2].

**SM2. Water height expression in the test for the spherical geostrophic equilibrium.** To define the initial water height, we assume that $h$ only depends upon latitude; i.e., $h(\varphi)$. Then, first and second equations of the 2D rotating shallow water equations on a sphere (2.1) are trivially satisfied since there are no longitudinal

*Submitted to the editors DATE.

**Funding:** This work was funded by Funded by ChEESE-2P (EU-EuroHPC JU-101093038) and DT-GEO project (HORIZON-INFRA-2021-TECH-01-01, number 101058129). This research has also been partially funded by MCIN/AEI/10.13039/501100011033 and by the "European Union NextGenerationEU/PRTR" through the Grant PDC2022-133663-C21 and by MCIN/AEI/10.13039/50110001103 and by "ERDF A way of making Europe," by the European Union through the Grant PID2022-137637NB-C21.

†Departamento de Análisis Matemático, Estadística e Investigación Operativa y Matemática Aplicada, Facultad de Ciencias, Universidad de Málaga, Campus de Teatinos, 29010 Málaga, Spain (alexgp@uma.es, mjcastro@uma.es, jmacias@uma.es).



*This manuscript is for review purposes only.*

variations in $h$. The third equation in (2.1), which represents the momentum balance, reduces to

$$-\left(\frac{Q_\theta^2}{Rh_\sigma\sigma}+\frac{gh_\sigma^2}{R\sigma^2}\right)\partial_\varphi\sigma+\frac{gh_\sigma\partial_\varphi h_\sigma}{R\sigma}=-fQ_\theta.$$

If we further assume $h \neq 0$, then this last equation is equivalent to

$$g\partial_\varphi h = -u_\theta^2\tan\varphi - Rfu_\theta. \tag{SM2.1}$$

Integrating equation (SM2.1) in the interval $[\varphi_0, \varphi]$ and using expression (5.5), the height is determined by the integral equation

$$h(\varphi) = h_0 - \frac{1}{g}\int_{\varphi_0}^{\varphi} R\,u_\theta(\xi)\left[2\,\Omega\sin\xi + \frac{\tan\xi}{R}u_\theta(\xi)\right]d\xi, \tag{SM2.2}$$

which can be approximated using a quadrature formula. We set $h_0 = 10100\,\mathrm{m}$ to be the global mean height.

## REFERENCES

[SM1] M. J. Castro, J. M. Gallardo, and A. Marquina, *A class of incomplete Riemann solvers based on uniform rational approximations to the absolute value function*, Journal of Scientific Computing, 60 (2013), pp. 363–389, https://doi.org/10.1007/s10915-013-9800-2.

[SM2] M. J. Castro, S. Ortega, and C. Parés, *Well-balanced methods for the shallow water equations in spherical coordinates*, Computers and Fluids, 157 (2017), pp. 196–207, https://doi.org/10.1016/j.compfluid.2017.08.035.

[SM3] M. J. Castro Díaz and E. Fernández-Nieto, *A class of computationally fast first order finite volume solvers: PVM methods*, SIAM Journal on Scientific Computing, 34 (2012), pp. A2173–A2196, https://doi.org/10.1137/100795280.

[SM4] A. Harten, P. D. Lax, and B. v. Leer, *On upstream differencing and Godunov-type schemes for hyperbolic conservation laws*, SIAM Review, 25 (1983), pp. 35–61, https://doi.org/10.1137/1025002.

[SM5] T. Morales de Luna, M. J. Castro Díaz, and C. Parés, *Relation between PVM schemes and simple Riemann solvers*, Numerical Methods for Partial Differential Equations, 30 (2014), pp. 1315–1341, https://doi.org/10.1002/num.21871.

[SM6] C. Parés, *Numerical methods for nonconservative hyperbolic systems: a theoretical framework*, SIAM Journal on Numerical Analysis, 44 (2006), pp. 300–321, https://doi.org/10.1137/050628052.

[SM7] E. F. Toro, M. Spruce, and W. Speares, *Restoration of the contact surface in the HLL-Riemann solver*, Shock Waves, 4 (1994), pp. 25–34, https://doi.org/10.1007/bf01414629.
